# Supplementary material for: VidTr: Video Transformer Without Convolutions
Source: arXiv:2104.11746 source file (2021-10-15)
Supplement: Supplementary file 1 [file Appendix.tex]

\clearpage
\appendix
% \appendixpage
\setcounter{figure}{0} 
\setcounter{table}{0}

\section{Compact-VidTr implementation details}
\label{appendix:implementation}
We provide some details for $topK_{std}$ pooling.
We calculate the row-wise standard deviation as:
\begin{flalign}
    \sigma^{(i)} & = \frac{1}{T}\sqrt{ \sum_{i=1}^{T} (Attn_t^{(i, :)} - \mu)^2} \\
    \mu^{(i)} &  = \frac{1}{T}\sum_{i=1}^{T} Attn_t^{(i, :)}
\end{flalign}
where $\sigma \in \mathbb{R}^{T}$ and $\mu \in \mathbb{R}^{T}$ are row-wise standard deviation, and mean of $Attn_t^{(1:,:)}$. Note that the $topK\_std$ pooling was applied to the affinity map excluded the token $Attn_t^{(1:,:)}$ as we will always preserve token for information aggregation. 

\section{Fast VidTr}
\label{appendix:fastvidtr}

As a common practice, 3D ConvNets are usually tested on 30 crops per video clip (3 spatial and 10 temporal) that show performance boost while greatly increase the computation cost.
The VidTr has been proved that learn long-term global spatio-temporal features better in a video clip, thus we propose to sample the data in TSN style (segment video into N chunks and randomly pick one frame from each chunk).
% and directly learn the spatio-temporal features from them.  
During testing, we uniformly sample N frames from the video regardless the length of the video, and perform single-pass inference (center crop). Such design significantly reduce the inference computation and latency caused by the dense sampling with a very small performance drop (about 2\%, see Table \ref{tab:k400_FI}). Note that the R2D and I3D based methods do not work well with sparsely sampled frames, mainly because the convolution kernel has limited receptive field and can only aggregate features slowly. If adjacent frames are too far away from each other, the temporal convolution will not be able to establish the temporal relations well. 
\begin{table}[h!]
    \footnotesize
	\begin{center}
		\begin{tabularx}{1\columnwidth}{l|c|c|c|c|c} 
		    \toprule
			Model        &Input & Res.& GFLOPs & Latency(ms) &  Top1  \\ 
			\midrule
% 			I3D50 \cite{yang2020temporal}   & $32\times2$ & 256 & $10\times167$   & $165\times10$ &   \\
			TSM \cite{lin2019tsm} & $8f$TSN & 256  & $330$   & $170$ & 74.1  \\
			3DEffi-B4 \cite{feichtenhofer2020x3d}& $16\times5$ & 224  & $69$   & NA & 72.4  \\
            TEINet \cite{liu_AAAI2020_TEINet} & $16\times4$ & 256 & $990$ & $1080$ & 74.9 \\
			X3D-M \cite{feichtenhofer2020x3d} & $16\times5$  & 224  & $47$   & $1100$ & 74.6  \\
			\midrule
			F-VidTr-S        & $8\times8$  & 224  & $1\times39$ & $37$ & 72.9 \\
			F-VidTr-M       & $16\times4$   & 224   & $1\times59$ & $53$ & 74.7 \\
			\bottomrule
		\end{tabularx}
	\end{center}
	\caption{Comparison of VidTr to other fast networks. All results from previous methods except for TEINet (30-crops) are based on 10 temporal crop and center spatial crop. The VidTr was achieved by uniformly sample 8/16/32 frames temporally and center-crop spatially. }
	\label{tab:k400_FI}
\end{table}
We compare our fast VidTr model with previous SOTA light-weight models including TSM, TEINet and models from architecture search such as X3D on Kinetics 400 dataset and report the FLOPs, the latency and top1 accuracy with 10 center crops (Table \ref{tab:k400_FI})
The results show that our proposed one-pass inference significantly outperforms the competitors with less FLOPs, lower latency and higher accuracy.
The Fast VidTr (16 frames) is able to outperform TSM (+0.6\% accuracy, 70\% less FLOPs, 68\% less latency); TEINet (-0.2\% accuracy, 94\% less FLOPs, 95\% less latency), also note that the reported TEINet score is based on 30 crop evaluation; and X3D-M (+0.1\% accuracy, 24\% more FLOPs, 96\% less latency). The results proves that the VidTr is able to aggregate long-term spatio-temporal features more effectively comparing the 3D ConvNets.
% Most previous methods rely on dense sampling to achieve reasonable performance, while our VidTr achieves same or better performance with one pass inference. This is mainly because the convolution kernel learns local information only and thus, the convolutions kernel cannot effectively aggregate information from frames sampled at high sample rate. 
It is worth mentioning that: 1. Even without considering the 10-crop evaluation required for ConvNets to achieve reported scores, the VidTr is still able to inference roughly at same speed comparing with TEINet and significantly faster than X3D. 2. X3D has low FLOPs but high latency mainly due to the heavily use of depth convolution.

\section{More Ensemble Results}
\label{appendix:ensemble}

We provide additional ensemble results on Kinetics 400 (Table \ref{tab:sup_K400_en}) and charades (Table \ref{tab:sup_charades_res}), showing that the VidTr and 3D convolution based models can be complementary to each other, ensemble VidTr and 3D convolution based network significantly outperform the ensemble of any two 3D convolution based models.
Our results show that the result level ensemble of I3D-101 and SOTA 3D model TPN-101 lead to about 1\% accuracy boost and result level ensemble of VidTr-S with TPN-101 lead to about 3\% performance boost. The similar conclusion can be draw from Charades on multi-label activities, where the ensemble of I3D-101 and CSN-152 only gives 2.8\%mAP boost, while ensemble of VidTr-L with CSN-152 lead to SOTA (4.8\%mAP boost over CSN-152) performance on Charades datasets.  

\begin{table}[h!]
\footnotesize
	\begin{center}
		\begin{tabularx}{\columnwidth}{l|c|c|l|c|c} 
		    \toprule
			Model        & input & Ensemble & input & Top1 & Top5 \\ 
			\midrule
			I3D50 \cite{yang_CVPR2020_TPN}    & $16\times4$  & - &- & 75.0 & 92.2  \\
			I3D101 \cite{yang_CVPR2020_TPN}   & $16\times4$  & -  &-& 77.4 & 92.7  \\
		    TPN101 \cite{yang_CVPR2020_TPN}   & $16\times4$ & -  & -&78.2 & 93.4 \\
		    \midrule
			I3D50 \cite{yang_CVPR2020_TPN}    & $16\times4$ & I3D101 &$16\times4$ & 77.7 & 93.2  \\
			TPN101\cite{yang_CVPR2020_TPN}    &$16\times4$  & I3D50 & $16\times4$ & 78.5 & 93.3  \\ %8x8
		    TPN101 \cite{yang_CVPR2020_TPN}   & $16\times4$  & I3D101 & $16\times4$  & 79.3 & 93.8  \\ %8x8
		    \midrule
			VidTr-S              & $8\times8$ & I3D50 & $16\times4$ &  79.4 & 94.0  \\
			VidTr-S              & $8\times8$ & I3D101 & $16\times4$ & 80.3 & 94.6 \\
			VidTr-S              & $8\times8$ & TPN101 & $16\times4$ & 80.5 &  94.8 \\
			\bottomrule
		\end{tabularx}
	\end{center}
	\caption{More ensemble results on Kinetics-400 dataset. We report top 1 and top5 accuracy (\%) on validation set.}
	\label{tab:sup_K400_en}
\end{table}

\begin{table}[h!]
\small
    \begin{center}
        \begin{tabularx}{\columnwidth}{l|c|c|c|c} 
	    \toprule
		Model        & Input & Res. & Ensemble  &  Chad \\ 
		\midrule
		I3D-Inception \cite{carreira2017quo} & 64 $\times$ 1 & 256 &-& 32.9\\
        % STRG \cite{wang2018videos} & 32 $\times$ 4 & 256 & -& 39.7\\
        % LFB \cite{wu2019long} & 32 $\times$ 4 & 256 &  -&42.5\\
        % Nonlocal-101 \cite{wang2018non} & 32 $\times$ 4 & 288 & -& 37.5\\
        % SF101-NL \cite{feichtenhofer2018slowfast} & (64 + 8) $\times$ 2 & 256 &-& 45.2\\
        % X3D \cite{feichtenhofer2020x3d} & 16 $\times$ 5 & 312  &-& 47.1\\
        SlowFast-101-NL$^{*}$ & 32 $\times$ 4 & 256  &-&  44.7 \\
        CSN-152$^{*}$ & 32 $\times$ 4 & 256  &-&  46.4 \\
        \midrule
        En-I3D-101 & 32 $\times$ 4 & 256 & I3D-50 & 42.1\\
        En-I3D-101 & 32 $\times$ 4 & 256 & SF-101 & 47.9\\
        En-I3D-101 & 32 $\times$ 4 & 256 & CSN-152 & 49.2\\
        \midrule
		En-VidTr-L & 32 $\times$ 4 & 224 & I3D-101 & 47.3 \\
		En-VidTr-L & 32 $\times$ 4 & 224 & SF-101 &  48.9\\
		En-VidTr-L & 32 $\times$ 4 & 224 & CSN-152 & 51.2 \\
		\bottomrule
	\end{tabularx}
    \end{center}
	\caption{Results on Charades dataset. The evaluation metrics are mean average precision (mAP) in percentage. $^{*}$ denotes the result that we re-produced.}
	\label{tab:sup_charades_res}
\end{table}

\section{Error Analysis Details}
\label{appendix:err_details}
We show the top 5 classes that gains performance boost from VidTr and top 5 classes that got reduced performance from VidTr. The results (Table \ref{tab:supp_error}) show that the I3D generally performance well on local and fast action while the VidTr works well on actions require long-term temporal information. For example, the VidTr achieved 21.2 \% accuracy improvement over I3D on ``catching fish'' that requires long-term information from the status when the fish is in water to the final status after the fish is caught (Figure \ref{fig:supp_error_ana_a}). The VidTr performs worse than I3D on the activities that rely on slight motions (e.g., playing guitar, and shaking head, Figure \ref{fig:supp_error_ana_b})
% \arthur{We will add figures of those classes to help reader better understand}

\begin{table}[h!]
    \subfloat[Top 5 classes that VidTr works better than I3D.]{
		\begin{tabularx}{0.85\columnwidth}{l|c} 
			\toprule
			Top 5 (+)        & Accuracy gain   \\ 
			\midrule
			 	making a cake     &   +26.0\%     \\ 
		        catching fish &  +21.2\%  \\ 
			    catching or throwing baseball    &   +20.8\%    \\ 
			    stretching arm & +19.1\%   \\ 
			    spraying & + 18.0 \%\\
			\bottomrule
		\end{tabularx}
    } \hfill
    \subfloat[Top 5 classes that I3D works better than VidTr.]{
	\begin{tabularx}{0.75\columnwidth}{l|c} 
		\toprule
		Top 5 (-) & Accuracy gain   \\ 
		\midrule
		 	shaking head & -21.7\%     \\ 
	        dunking basketball &    -20.8\%  \\ 
		    lunge  & -19.9\%   \\ 
		    playing guitar &   -19.9\%  \\ 
		    tap dancing & -16.3\%\\
		\bottomrule
	\end{tabularx}
    } \hfill
	\caption{ Quantitative analysis on Kinetics-400 dataset. The performance gain is defined as the disparity of the top-1 accuracy between VidTr network and that of I3D.}
	\label{tab:supp_error}
\end{table}

\begin{figure}[h!]
    \subfloat[video examples that VidTr performs better than I3D..]{
    	\begin{center}
    	    \includegraphics[width=\columnwidth]{fig/fig_a_1_a.png}
    	\end{center}
    \label{fig:supp_error_ana_a}
	} 
	
    \subfloat[video examples that VidTr performs worse than I3D.]{
	\begin{center}
	    \includegraphics[width=\columnwidth]{fig/fig_a_1_b.png}
	\end{center}
    \label{fig:supp_error_ana_b}
	} 
	\caption{Visualizations of video samples that VidTr works better and I3D works better.
	}
\end{figure}

\section{Visualization Details}
\label{appendix:vis}

We visualized the VidTr's separable-attention with attention roll-out method \cite{abnar2020quantifying}. We multiplied all the affinity matrices between every two encoder layers and get $mask_{t} \in \mathbb{R}^{(WH + 1) \times (T + 1) \times (T + 1)}$ for the temporal roll-out attention and $mask_{s} \in \mathbb{R}^{(T + 1) \times (WH + 1) \times (WH + 1)}$ for the spatial roll-out attention. We selected the rows of class token from the roll-out attention for visualization as:
\begin{flalign}
    mask_{t}^{'} &= mask_{t}^{(1:, 0, 1:)} \in \mathbb{R}^{WH \times T}\\
    mask_{s}^{'} &= mask_{s}^{(1:, 0, 1:)} \in \mathbb{R}^{T \times WH}
\end{flalign}
We multiplied $mask_{t}^{'}$ and $mask_{s}^{'}$ to represent the spatial-temporal attention for visualize as:
\begin{equation}
    mask_{st}^{'} = Re(mask_{t}^{'}) \times mask_{s}^{'}
\end{equation}
where $mask_{st}^{'}$ is the spatio-temporal attention for visualize, and $Re$ denotes a reshape function. We threshold $mask_{s}^{'}$ and $mask_{st}^{'}$ by only highlighting the top 30\% of values of them, and attached them onto the original frames for visualizing the spatio-only and spatio-temporal attentions.

\subsection{More Visualizations}
We first show more results of the VidTr's separable-attention with attention roll-out method \cite{abnar2020quantifying} (Figure \ref{fig:supp_vis_1}). We find that the spatial attention is able to focus on informative regions and temporal attention is able to skip the duplicated/non-representative information temporally.

\begin{figure*}[h!]
    \begin{center}
    	    \includegraphics[width=0.92\textwidth]{VidTr/fig/supp_vis_1_1.png}
    	    
    	    \vspace{5mm}
    	    
    	    \includegraphics[width=0.92\textwidth]{VidTr/fig/supp_vis_1_2.png}
    	    
    	    \vspace{5mm}
    	    
    	    \includegraphics[width=0.92\textwidth]{VidTr/fig/supp_vis_1_3.png}
	\end{center}
	\caption{The spatial and temporal attention in Vidtr. The attention is able to focus on the informative frames and regions.
	}
	\label{fig:supp_vis_1}
\end{figure*}

We then show more results of the attention at 4th, 8th and 12th layer of VidTr (Figure \ref{fig:supp_vis_2}), 
we found the spatial attention is getting to concentrate better  when it goes to the deeper layer.
The attention did not capture meaningful temporal instances at early stages because the temporal feature relies on the spatial information to determine informative temporal instances. 

\begin{figure*}[h!]
    \begin{center}
    	    \includegraphics[width=0.8\textwidth]{VidTr/fig/supp_vis_2_1.png}
    	    
    	    \vspace{4mm}
    	    
    	    \includegraphics[width=0.8\textwidth]{VidTr/fig/supp_vis_2_2.png}
    	    
    	    \vspace{4mm}
    	    
    	    \includegraphics[width=0.8\textwidth]{VidTr/fig/supp_vis_2_3.png}
	\end{center}
	\caption{The rollout attentions from different layers of VidTr.
	}
	\label{fig:supp_vis_2}
\end{figure*}

Finally we compared the I3D activation map and rollout attention from VidTr (Figure \ref{fig:supp_vis_3}). The I3D mis-classified the catching fish as sailing, as the I3D attention focused on the people sitting behind and water. The VidTr is able to make the correct prediction and the attention showed that the VidTr is able to focus on the action related regions across time.

\begin{figure*}[h!]
    \begin{center}
    	    \includegraphics[width=0.9\textwidth]{VidTr/fig/supp_vis_3_1.png}
    	    
    	    \vspace{5mm}
    	    
    	    \includegraphics[width=0.9\textwidth]{VidTr/fig/supp_vis_3_2.png}
    	    
            \vspace{5mm}
    	    
    	    \includegraphics[width=0.9\textwidth]{VidTr/fig/supp_vis_3_3.png}	
    \end{center}
	\caption{Comparison of I3D activations and VidTr attentions.
	}
	\label{fig:supp_vis_3}
\end{figure*}
